# Supplementary material for: The Nun Path: The Evolution and Quenching of Satellite Galaxies
Source: arXiv:2103.10258 source file (2021-03-18)
Supplement: Supplementary file 1 [file app0A.tex]

%
% file: app0A.tex
% author: Tomer Nussbaum
% description: ?
%
% 
\chapter{Elliptical galaxy formation (eCg) }
\label{app:app01}

\initial{W}e present here \textbf{preliminary} additional visualizations regarding SG 22-004, the eCg case.

The galaxy was formed in a filament, the full filament is hard to observe via 2d picture. Therefore we supply a 3D interactive model of the filament. Available here: 
\textcolor{blue}{\href{https://skfb.ly/6wxpS}{Filament Model}} When the surfaces are iso-densities contours of the filament. Fig~\ref{fig:Formation_in_filament} presents the first identification snapshot and Fig~\ref{fig:eCg_example} present the SG evolution product, an eCg.

Also we provide here five \textbf{preliminary} 3D-models representing different stages in the SG 22-004 evolution: 
\cite{Kiyun2019} jellyfish

1. Entering Rvir
2. Contraction & sSFR decrease - https://skfb.ly/6wwnn
3. Mid sSFR - https://skfb.ly/6wwnn
4. No sSFR - https://skfb.ly/6wwus
5. Sigma 0.5kpc fall

\begin{figure}[H] \centering
\includegraphics[width=0.9\linewidth]{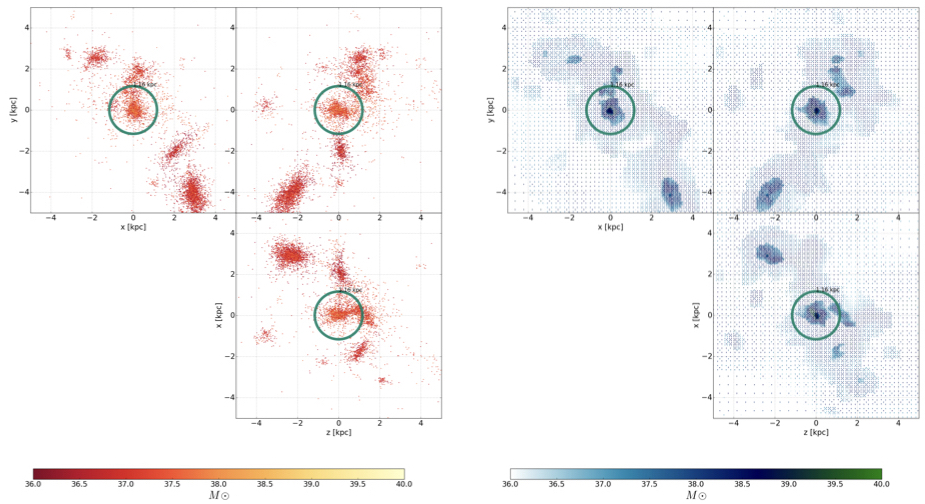}
\includegraphics[width=0.9\linewidth]{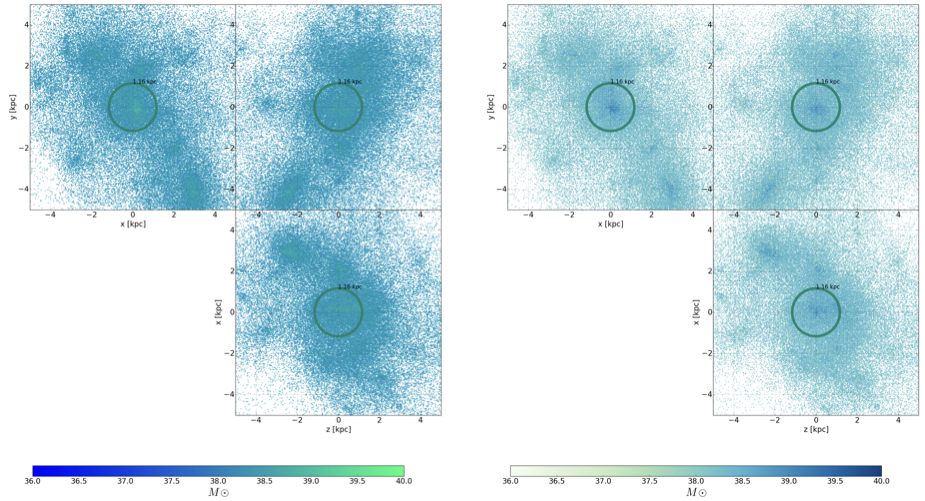}	\caption{\small \textbf{Formation in a filament, gas rich environment} 
The figure is divided to 4 plots, each of them shows a different projected mass quantity. from left to right, up then down: stars, gas, dark matter and total mass. colored is the summed mass in a cell. Note that each subplot is divided to three subsubplots, they represent different projections, y-x,y-z,x-z, in order to grasp the 3d shape of the galaxy. The circle represent the approximated $R_{\textrm sat}$.
\hspace{0.5} The figure shows the eCg first identification snapshot at the VELA simulation before it was. we can see the formation moment of the SG in a very high dense gas region inside a filament. }
 \label{fig:Formation_in_filament}
\end{figure}

\begin{figure}[H] \centering
\includegraphics[width=0.9\linewidth]{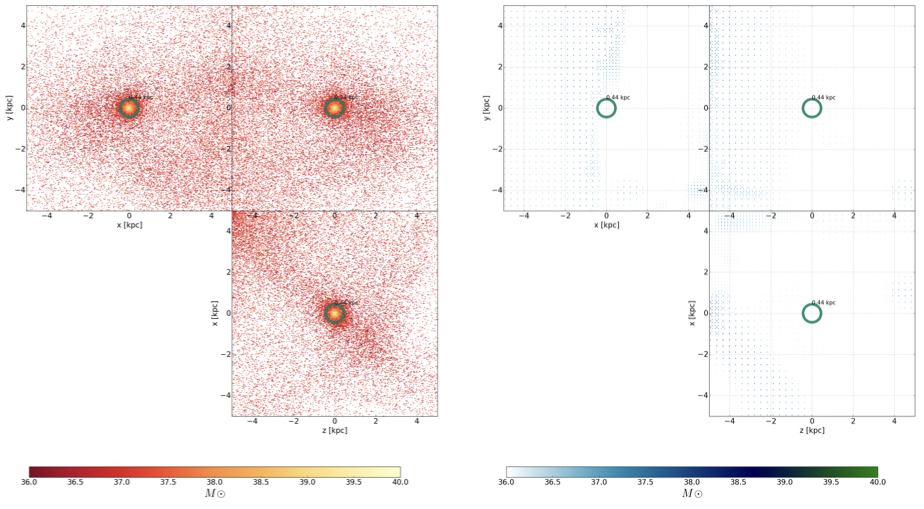}
\includegraphics[width=0.9\linewidth]{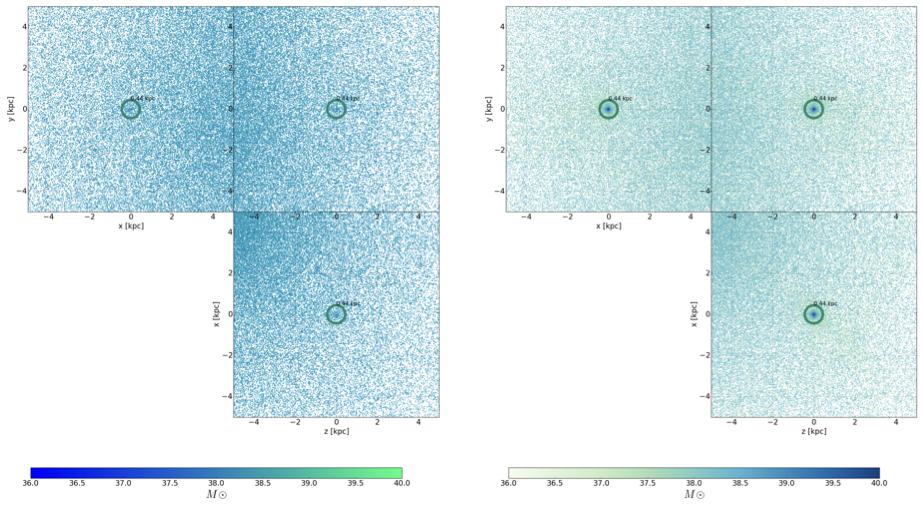}
\caption{\small \textbf{eCg example} 
Colors and methods are similar to Fig.~\ref{fig:fig:Formation_in_filament}
\hspace{0.5} In this figure we can see a clear elliptical compact galaxy without gas or dark matter}
\label{fig:eCg_example}
\end{figure}

\textcolor{red}{3D model}
filament, 1,2,3,4,5

% \textcolor{red}{Maybe add UDG which losses all its dark matter}
